# Supplementary material for: Prediction and control of geometry-induced nematic order in growing multicellular systems
Source: arXiv:2506.10867 ancillary file (2025-06-12)
Supplement: Supplementary file 1 [file supplement.pdf]

# Supplementary Material for "Prediction and control of geometry-induced nematic order in growing multicellular systems"

Lukas Hupe,[1,2] Jonas Isensee,[1,2] Ramin Golestanian,[1,2,3] and Philip Bittihn[1,2,*]

[1]Max Planck Institute for Dynamics and Self-Organization, Göttingen, Germany
[2]University of Göttingen, Institute for Dynamics of Complex Systems, Göttingen, Germany
[3]Rudolf Peierls Centre for Theoretical Physics, University of Oxford, Oxford OX1 3PU, United Kingdom

## I. AGENT-BASED NUMERICAL MODEL

As stated in the main text, we use one of the two models introduced in Ref. 1, which describes individual cells as spherocylinders of width 1 that grow in length with a constant rate and divide into two equal halves when reaching their division length $l^{\max}$, here set to 2, except where otherwise noted. Particles interact sterically, with repulsion force scaling with the 1.5th power of the largest overlap distance between two rods, measured orthogonally to their perimeter. This interaction is scaled by the cell Young's modulus $Y$, which we generally set to a value of $5 \cdot 10^6$ to stay close to the incompressible limit. Particle mobilities scale with cell bounding box area, i.e., the product of cell width $w$ and length $l$ (including the semicircular caps), and a specific friction $\eta$, with

$$\mu^{\text{trans}} = \frac{1}{w\,l\,\eta} \text{ and } \mu^{\text{rot}} = \frac{12\mu^{\text{trans}}}{4R^2 + l^2}, \tag{S1}$$

where $\mu^{\text{trans}}$ and $\mu^{\text{rot}}$ are the translational and rotational mobilities respectively. For all simulations in this work, we set $\eta = 0.3$.

Equations of motions are integrated with an Euler integrator, using an adaptive time stepping scheme, which uses a heuristic to restrict the maximum displacement in a single time step to 0.005 length units, while additionally capping time steps at $10^{-4}$ time units. All parameter sets are simulated for 16 realisations, with ensemble averages applied to produce the alignment fields presented in the main text.

## II. QUANTIFYING ORDER AND ALIGNMENT

In the main text, we use a scalar product order parameter $q_{\text{rad}} = 2\left\langle (\hat{\mathbf{n}} \cdot \hat{\mathbf{r}})^2 \right\rangle - 1$ to quantify nematic order along a specified direction. Here, we show how this order parameter relates to the nematic tensor $\underline{\mathbf{Q}}$, which enables us to exploit the radial symmetry to rewrite the tensorial equation for $\underline{\mathbf{Q}}$ as a scalar ODE for $q_{\text{rad}}$.

Using a statistical definition of $\underline{\mathbf{Q}}$ for an ensemble of directors $\hat{\mathbf{n}}$, and applying it to the radial unit vector field $\hat{\mathbf{r}}(\mathbf{r})$ , we obtain

$$\underline{\mathbf{Q}}(\mathbf{r})\,\hat{\mathbf{r}}(\mathbf{r}) = \left( \langle \hat{\mathbf{n}}(\mathbf{r}) \otimes \hat{\mathbf{n}}(\mathbf{r}) \rangle_{\text{ensemble, time}} - \frac{\underline{\mathbf{I}}}{2} \right) \hat{\mathbf{r}}(\mathbf{r}) \tag{S2}$$

$$= \langle (\hat{\mathbf{n}} \otimes \hat{\mathbf{n}})\;\hat{\mathbf{r}} \rangle - \hat{\mathbf{r}}/2 \tag{S3}$$

$$= \langle (\hat{\mathbf{n}} \cdot \hat{\mathbf{r}})\;\hat{\mathbf{n}} \rangle - \hat{\mathbf{r}}/2 \tag{S4}$$

As we are interested in an expression for $\left\langle (\hat{\mathbf{n}} \cdot \hat{\mathbf{r}})^2 \right\rangle$, we now multiply our result with $\hat{\mathbf{r}}$, yielding

$$\left\langle (\hat{\mathbf{n}} \cdot \hat{\mathbf{r}})^2 \right\rangle = (\underline{\mathbf{Q}}\hat{\mathbf{r}}) \cdot \hat{\mathbf{r}} + 1/2\,. \tag{S5}$$

From radial symmetry, we know that $\underline{\mathbf{Q}}$ must be of the form $q(r)\,(\hat{\mathbf{r}} \otimes \hat{\mathbf{r}} - \underline{\mathbf{I}}/2)$ with a radial dependency $q(r)$. Inserting this into Equation (S5), we get

$$\left\langle (\hat{\mathbf{n}} \cdot \hat{\mathbf{r}})^2 \right\rangle = \frac{q(r) + 1}{2},$$

which can be rearranged to show that the scalar product order parameter $q_{\text{rand}}$ as defined in the main text is equal to $q(r)$. This argument also applies in the channel limit, with the radial axis replaced with the channel axis in the definition of the order parameter and $\underline{\mathbf{Q}}$.

## III. PRESSURE, VELOCITY AND SHEAR RATE IN RADIALLY SYMMETRIC COLONIES

### A. General solution

We consider an isotropically expanding incompressible material with constant expansion rate $\alpha$, growing in a radially symmetric domain. We aim to derive the growth-generated pressure field $p$, the flow field $\mathbf{v}(\mathbf{r})$ and shear rate tensor $\underline{\mathbf{u}}^{\text{ST}}(\mathbf{r})$.

We begin with a Poisson equation for the pressure field

$$\nabla^2 p = -\frac{\alpha}{\zeta}\,. \tag{S6}$$

where $\zeta$ is the effective mobility of the colony. At the inner boundary $R_0$ we impose a constant injection velocity boundary condition, with

$$(\nabla p \cdot \hat{\mathbf{r}})\big|_{r=R_0} = -\frac{1}{\zeta}\mathbf{v} \cdot \hat{\mathbf{r}}\Big|_{r=R_0} = -\frac{v_0}{\zeta}\,, \tag{S7}$$

At the outer boundary at radius $R_1 = R_0 + \Delta R$, we introduce a zero-pressure boundary condition, corresponding to the absorbing boundaries in the agent-based system.

* philip.bittihn@ds.mpg.de

We can make use of the radial symmetry of the system to simplify (S6) to 1D, yielding

$$\frac{\partial^2}{\partial r^2} p + \frac{1}{r}\frac{\partial}{\partial r} p + \frac{\alpha}{\zeta} = 0\,. \tag{S8}$$

The solution to the homogeneous part of this equation is $c_1 + c_2 \log(r)$, the inhomogeneous problem is solved by $-\alpha r^2/4\zeta$. We insert the boundary conditions: the Neumann condition at $R_0$ sets

$$c_2 = \frac{\alpha R_0^2}{2\zeta} - \frac{R_0 v_0}{\zeta}\,, \tag{S9}$$

while the Dirichlet condition at $R_1$ sets

$$c_1 = \frac{\alpha R_1^2}{4\zeta} - c_2 \log(R_1)\,. \tag{S10}$$

We can now combine all of these results into a general solution for the pressure profile:

$$p = \frac{\alpha R_1^2}{4\zeta} + \left(\frac{\alpha R_0^2}{2\zeta} - \frac{R_0 v_0}{\zeta}\right)\log\left(\frac{r}{R_1}\right) - \frac{\alpha r^2}{4\zeta} \tag{S11}$$

$$= \frac{\alpha}{4\zeta}\left[R_1^2 + 2R_0^2 \log\left(\frac{r}{R_1}\right) - r^2\right] - \frac{R_0 v_0}{\zeta}\log\left(\frac{r}{R_1}\right)\,. \tag{S12}$$

Using $\mathbf{v} = -\zeta \nabla p$, we take the gradient of Eq. S12 to arrive at the flow field

$$\mathbf{v}(\mathbf{r}) = \left(\left(\frac{v_0}{R_0} - \frac{\alpha}{2}\right)\left(\frac{R_0}{r}\right)^2 + \frac{\alpha}{2}\right)\mathbf{r}\,. \tag{S13}$$

Setting $v_0 = 0$ and $R_0 \to 0$ corresponds to the case of isotropic Hubble-like growth with the expected linear radial velocity profile with gradient $\alpha/2$. Other values of $R_0$ or $v_0$ create deviations from this profile that decay with increasing radius.

Taking the gradient again, we can also compute the shear rate tensor $\underline{\mathbf{u}}^{\mathrm{ST}}$

$$\underline{\mathbf{u}}^{\mathrm{ST}} = d\left(\frac{\alpha}{2} - \frac{v_0}{R_0}\right)\left(\frac{R_0}{r}\right)^2\left(\hat{\mathbf{r}} \otimes \hat{\mathbf{r}} - \frac{\underline{\mathbf{I}}}{2}\right)\,. \tag{S14}$$

We see that this expression can only be nonzero for $R_0 \neq 0$, and changes sign depending on the injection velocity $v_0$.

### B. Zero curvature limit

We want to make sure that in the limit of zero curvature ($R_0 \to \infty$ with fixed $\Delta R$), these results are consistent with the solution for simple one-dimensional channel flow. In order to take this limit without losing our variable $r$ to infinity, we first express $p$ in terms $x = r - R_0$, the distance from the inner boundary:

$$p = \frac{\alpha}{4\zeta}\left[\Delta R^2 - x^2 + 2R_0\left(\Delta R - x + R_0 \log\left(\frac{R_0 + x}{R_1}\right)\right)\right] - \frac{R_0 v_0}{\zeta}\log\left(\frac{R_0 + x}{R_1}\right)\,. \tag{S15}$$

At this point, it is pertinent to spend some time on computing the limit $\lim_{x\to\infty} x \log\left(\frac{x+a}{x+b}\right)$. For this, we expand the expression for $a$ and $b \ll x$. We compute the relevant partial derivatives

$$\frac{\partial^n}{\partial a^n} x \log\left(\frac{x+a}{x+b}\right) = (-1)^{n-1}(n-1)!\frac{x}{(x+a)^n} \tag{S16}$$

$$\frac{\partial^n}{\partial a^n} x \log\left(\frac{x+a}{x+b}\right) = (-1)^{n}(n-1)!\frac{x}{(x+b)^n}\,, \tag{S17}$$

noting that all cross-terms $\frac{\partial^{n+m}}{\partial a^n \partial b^m}$ vanish here and that in the limit of $x \to \infty$, only the first-order term of the expansion can have non-zero coefficients. From this, we deduce

$$\lim_{x\to\infty} x \log\left(\frac{x+a}{x+b}\right) = a - b \tag{S18}$$

We apply this result to the injection-driven term of the pressure profile, which approaches $(v_0/\zeta)(\Delta R - x)$ in the zero-curvature limit. This result is consistent with expectations as it corresponds to a constant offset of $v_0$ to the flow velocity.

The growth-driven term of the pressure profile consists of a parabolic term which is independent of $R_0$, and a curvature-dependent correction of the form

$$\frac{\alpha}{2\zeta} R_0\left(\Delta R - x + R_0 \log\left(\frac{R_0 + x}{R_0 + \Delta R}\right)\right)\,. \tag{S19}$$

Naively, the presence of the linear term $R_0(\Delta R - x)$ could lead to the assumption that this expression must necessarily diverge. However, we can show using our previously acquired knowledge (Eq. S18) that the entire bracketed term vanishes for $R_0 \to \infty$.

To compute the value of the limit, a similar argument from a polynomial expansion up to second order can be applied. This calculation results in the familiar term

$$\lim_{x\to\infty} \frac{\alpha}{2\zeta} R_0\left(\Delta R - x + R_0 \log\left(\frac{R_0 + x}{R_0 + \Delta R}\right)\right) = \frac{\alpha}{4\zeta}(\Delta R^2 - x^2)\,, \tag{S20}$$

and thus in the limit for the total stress profile

$$\boxed{\lim_{R\to\infty} p(x) = \frac{\alpha}{2\zeta}\left(\Delta R^2 - x^2\right) + \frac{v_0}{\zeta}(\Delta R - x)\,.} \tag{S21}$$

For $v_0 = 0$, this result reproduces the parabolic stress field and linear velocity profile with gradient $\alpha$, consistent with the known results for rectangular channels.

### C. Central pressure

From these results we can now extract the "central" stresses (i.e. $p$ at $R_0$) for the case $v_0 = 0$ as

$$p_0 = \frac{\alpha}{4\zeta}\left[\Delta R^2 + 2R_0\left(\Delta R + R_0 \log\left(\frac{R_0}{R_1}\right)\right)\right]\,, \tag{S22}$$

with the limits

$$\boxed{\begin{aligned}\lim_{R_0\to 0} p_0 &= \frac{\alpha \Delta R^2}{4\zeta}\\ \lim_{R_0\to\infty} p_0 &= \frac{\alpha \Delta R^2}{2\zeta}\end{aligned}} \tag{S23}$$

We notice that in the $R_0 \to 0$ limit, where the material is free to expand in two dimensions, central pressure is half as high as in the case of $R_0 \to \infty$, where the material can only expand along one axis.

### D. Effects of nonuniform density

All results up to this point assume incompressibility of the colony; in fact the Poisson equation for $p$ is derived from an equation of continuity with constant density, as explained in the main text. However, in our numerical simulations, cells have finite hardness by necessity, further limited by performance considerations: Increasing cell hardness requires smaller time steps, thus directly increasing simulation runtimes.

Therefore, cell densities in our simulations are generally vary slightly, with density decreasing towards open boundaries. Here, we will attempt to qualitatively understand the influence of these nonuniformities on the shear rate tensor. For this we introduce a density term $\rho$ into the continuity equation, i.e.

$$\frac{\partial}{\partial t}\rho + \nabla \cdot \rho \mathbf{v} = \alpha \rho \,. \tag{S24}$$

Fully solving this equation would require an additional equation of state, linking density to mechanical stresses. Therefore, we here measure the number densities in agent-based simulations and approximate the steady state function with a biquadratic polynomial (Fig. S5a) to obtain a qualitative estimate. Using numerical integration, we can obtain a velocity profile (Fig. S5b) and shear rate magnitude (Fig S5c). While the corrected velocity profiles are visually hard to distinguish from the constant-density approximation, the difference is much more pronounced for the shear rates: Close to $R_1$, the magnitude of $\underline{\mathbf{u}}^{\mathrm{ST}}$ increases faster than predicted by Eq. S14, reminiscent of the trumpet-like shape observed in the agent-based simulations (main text, Fig. 4).

## IV. PRESSURE, VELOCITY AND SHEAR RATE IN OPEN EQUILATERAL TRIANGULAR SYSTEMS

As a basic example for a domain with "corners", we consider an equilateral triangle with height $h$. The geometry is not simple enough in any coordinate system to write down an ansatz for the velocity field that respects the symmetries and can automatically satisfy the zero-stress boundary conditions, so we have to solve explicitly for the stress (pressure). For this, we make the same assumptions of isotropic growth as in the main text, thus arriving at a simple Poisson equation for the pressure. As we are only interested in the flow field, we assume a mobility of 1 without loss of generality, thus reducing the equation to

$$\nabla \cdot \mathbf{v} = -\nabla^2 p = \alpha \tag{S25}$$
$$\text{with } p = 0 \text{ on } \partial D,$$

where $D$ is the domain. It can be shown that the equilateral triangle is the only polygon for which algebraic solutions of the Poisson problem exist [2]. If we place one corner at the origin and one side at $y = h$, such that points on the other two sides satisfy $y = \pm\sqrt{3}x$, this solution reads [2]

$$p(x, y) = -\frac{\alpha}{4}(3x^2 - y^2)\left(1 - \frac{y}{h}\right). \tag{S26}$$

From this solution, which is shown in Figure S1, we can then

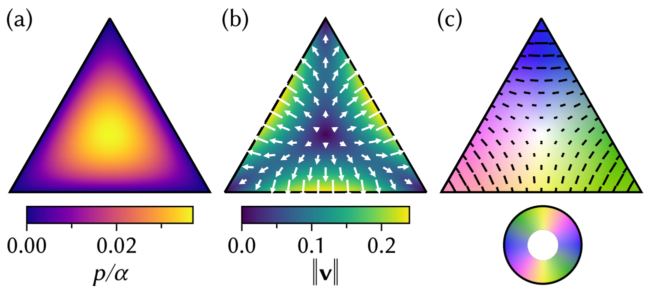


Figure S1. Solution for isotropic growth in an open equilateral triangle. (a) Pressure. (b) Flow field. (c) Characteristics of the shear rate, with the principle direction of $\underline{\mathbf{u}}^{\mathrm{ST}}$ indicated by black bars and the color code, whereas intensity indicates the strength of the shear-induced alignment $S = |\underline{\mathbf{u}}^{\mathrm{ST}}|$. The total topological charge in the domain is $-1/2$.

calculate $\mathbf{v} = -\nabla p$ and $\underline{\mathbf{u}}^{\mathrm{ST}}$. After some algebra, we arrive at

$$\mathbf{v} = \frac{\alpha}{2}\left(3x\left(1 - \frac{y}{h}\right), \; \frac{3y^2 - 3x^2}{2h} - y\right)^{\mathrm{T}} \tag{S27}$$

$$\underline{\mathbf{u}}^{\mathrm{ST}} = \alpha \begin{pmatrix} 1 - \frac{3y}{2h} & -\frac{3x}{2h} \\ -\frac{3x}{2h} & \frac{3y}{2h} - 1 \end{pmatrix}, \tag{S28}$$

where, consistent with the symmetry of the problem, we find no shear in the center of the triangle at $(x, y) = (0, 2h/3)$. Because of this symmetry, we can also examine the behavior around the boundary by looking at shear rate tensor in an arbitrary corner and in the middle of an arbitrary side. In the middle of the upper side at $(x, y) = (0, h)$, we have

$$\underline{\mathbf{u}}^{\mathrm{ST}}(0, h) = \alpha \begin{pmatrix} -1/2 & 0 \\ 0 & 1/2 \end{pmatrix}, \tag{S29}$$

corresponding to a bias towards an orientation in the $y$ direction, i.e. perpendicular to the side (or "radially" in the relation to the center). In contrast, at the downward pointing tip of the triangle at $(x, y) = (0, 0)$, we have

$$\underline{\mathbf{u}}^{\mathrm{ST}}(0, 0) = \alpha \begin{pmatrix} 1 & 0 \\ 0 & -1 \end{pmatrix}, \tag{S30}$$

which corresponds to a bias towards horizontal alignment (or "tangentially" relative to the center). We can also see that the bias is stronger in the corners.

Assuming that the steady-state alignment field is proportional to the shear rate, we can reinterpret $\underline{\mathbf{u}}^{\mathrm{ST}}$ as a $\underline{\mathbf{Q}}$ tensor. This allows us to compute the director, and from

that the topological charge. The angle $\phi$ of the director $\mathbf{n} = (\cos\phi, \sin\phi)$ can then be calculated in a straight-forward manner as

$$\tan\phi(x,y) = \frac{Q_{xy}}{Q_{xx}+S/2} = -\frac{x/y}{\frac{2h}{3y} - 1 + \sqrt{(x/y)^2 + (\frac{2h}{3y}-1)^2}}. \tag{S31}$$

We then integrate along the boundary of the domain to calculate the topological charge. Along the most convenient top side at $y = h$, we have

$$\frac{\mathrm{d}}{\mathrm{d}t}\phi(x(t),h) = -\frac{\sqrt{3}}{4+12(t-1)t}, \tag{S32}$$

where $x(t) = h(1-2t)/\sqrt{3}$ parametrises the path along the side. Because of symmetry, the contribution must be the same from all three sides, such that the total topological charge is

$$\frac{1}{2\pi}\oint \mathrm{d}\phi = \frac{3}{2\pi}\int_0^1 \frac{\mathrm{d}\phi}{\mathrm{d}t}\,\mathrm{d}t = -\frac{1}{2}. \tag{S33}$$

The orientation changes repeatedly from radial in the middle of the sides to tangential at the corners, but the radial orientation itself does a full revolution in the positive direction, leading to a net charge of $-1/2$. This can also be read off from Figure S1c.

## V. FULL SOLUTION TO THE ADVECTION DECAY MODEL

The full solution to the advection decay model on a ring geometry, including an injection velocity $v_0$ at the inner radius, is given by

$$q(r) = q_0\,{}_2F_1\left(1, \tfrac{\mu}{\alpha}; 1+\tfrac{\mu}{\alpha}; \tfrac{f(r)}{2R_0v_0-\alpha R_0^2}\right) + C\,f(r)^{-\frac{\mu}{\alpha}} \tag{S34}$$

with $f(r) = \alpha\left(r^2 - R_0^2\right) + 2R_0v_0$ and a constant $c$. We impose a fixed boundary condition $q(R_0) = q_{in}$ and obtain

$$q(r) = q_0\,{}_2F_1\left(1, \tfrac{\mu}{\alpha}; 1+\tfrac{\mu}{\alpha}; \tfrac{f(r)}{2R_0v_0-\alpha R_0^2}\right) - \left(\frac{f(r)}{2R_0v_0}\right)^{-\frac{\mu}{\alpha}}\left(q_0\,{}_2F_1\left(1, \tfrac{\mu}{\alpha}; 1+\tfrac{\mu}{\alpha}; \tfrac{f(R_0)}{2R_0v_0-\alpha R_0^2}\right) - q_{in}\right) \tag{S35}$$

We note that in the case of $v_0 = 0$, corresponding to the ring system discussed in the main text, the term $2R_0v_0/f(r)$ is zero for all $r \neq R_0$, confirming our assumption that in this case the homogeneous solution cannot play a role in the bulk.

## VI. SUPPLEMENTARY FIGURES

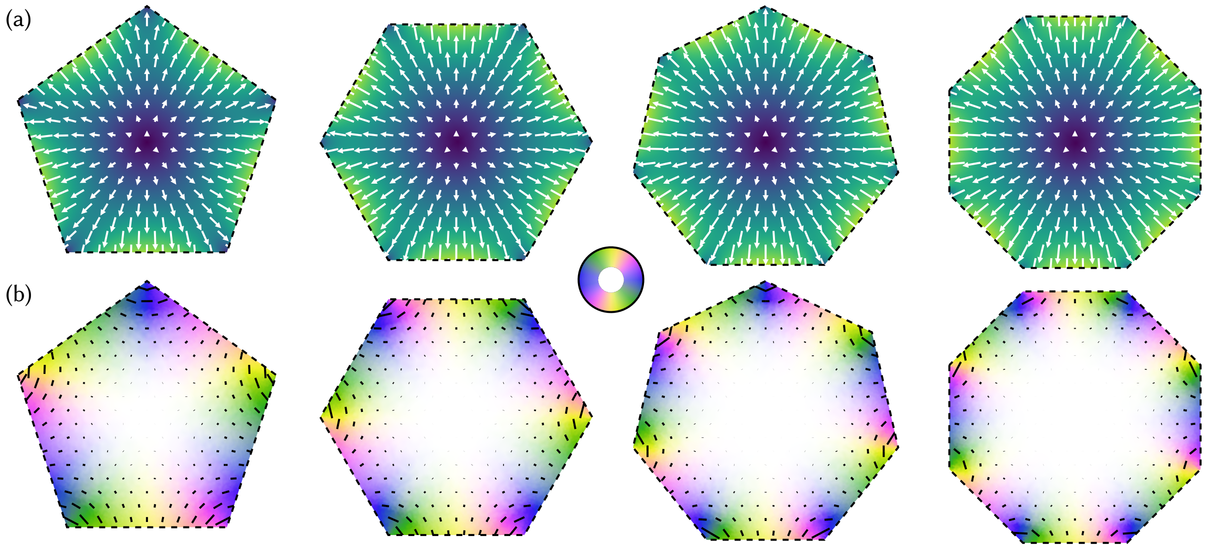


Figure S2. (a) Velocity fields for constant expansion flow in various polygonal domains, computed by solving Eq. 2in the main text using finite element methods. (b) Principal direction and magnitude of the shear rate tensor of the flow fields in panel a.

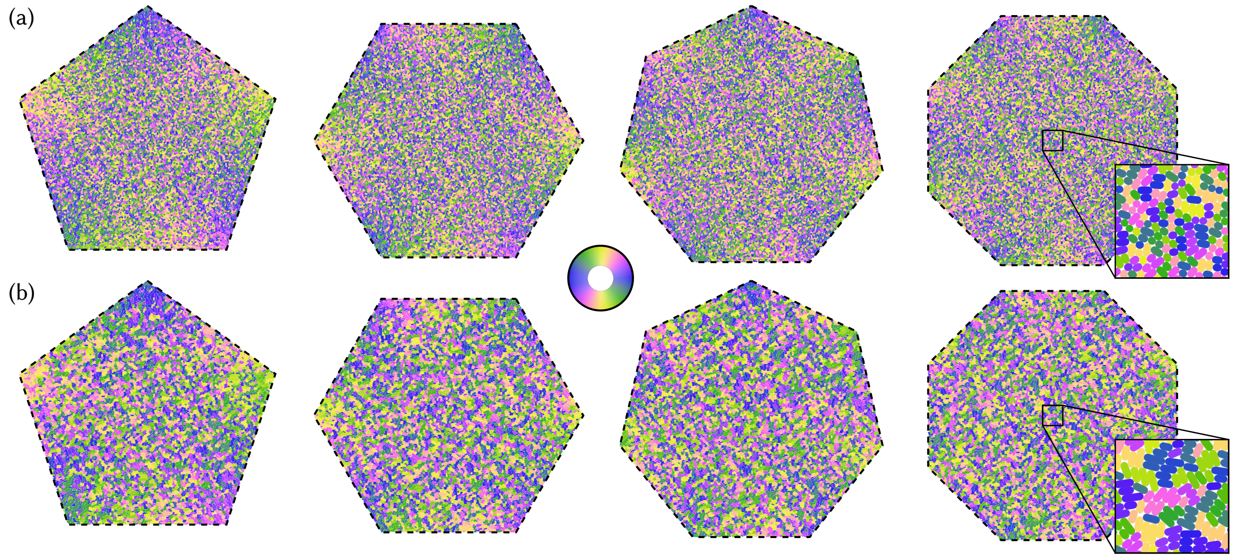


Figure S3. (a) Snapshots of agent-based simulations of growing colonies in various polygonal domains with escribed radii of 100 units, with division aspect ratio 2. Cells are color-coded by domain. Inset shows a $15 \times 15$ section of the colony. (b) Same as panel a, for cells of division aspect ratio 3.

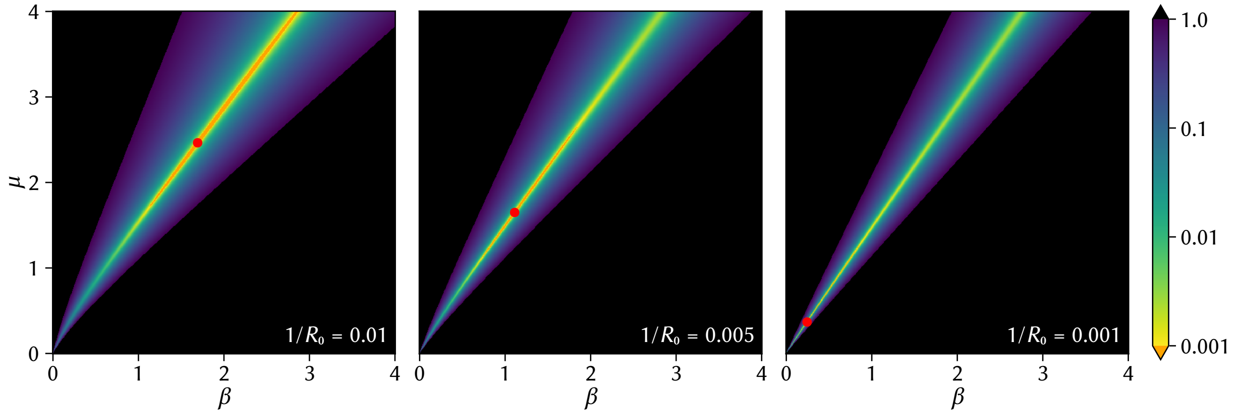


Figure S4. Fit landscapes for the advection-decay model fits shown in Fig. 4 in the main text. Color-coded plots show mean squared difference between theory and numerics for different values of $\beta$, $\mu$, shifted by the residual so that the field vanishes at the best-fit values (red marker).

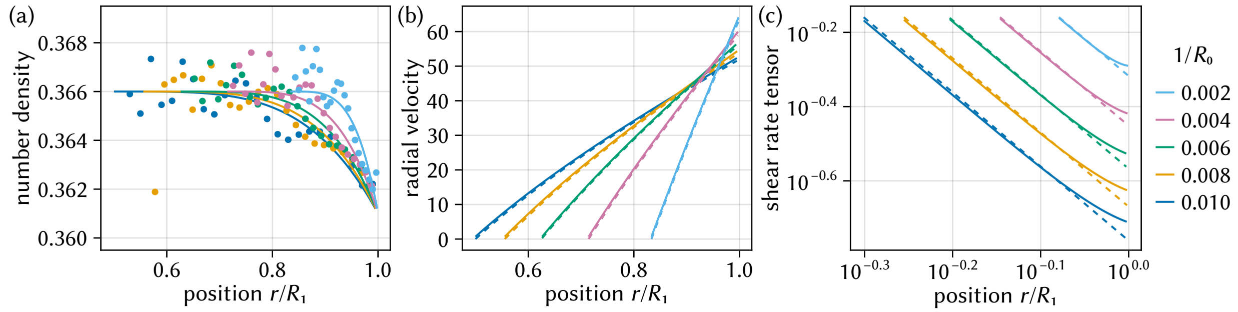


Figure S5. (a) Number density profiles for the ring systems in Fig. 4 (dots), with parabolas for $\rho_0 = 0.361$ and $\delta_\rho = 0.005$. (b) Theoretical velocity profile with (solid lines) and without (dashed lines) density correction following the parabolas in panel a. (c) Theoretical shear rate tensor magnitude, with and without density correction as in panel b.

[1] Lukas Hupe, Yoav G. Pollack, Jonas Isensee, Aboutaleb Amiri, Ramin Golestanian, and Philip Bittihn. A minimal model of smoothly dividing disk-shaped cells, September 2024.
[2] E. A. Volkov. On a Property of Solutions to the Poisson Equation on Polygons. *Math Notes*, 66(2):139–141, August 1999.
